# Supplementary material for: Exploring Unconfirmed Transactions for Effective Bitcoin Address Clustering
Source: arXiv:2303.01012 source file (2023-03-03)
Supplement: Supplementary file 1 [file 08_Appendix.tex]

\appendix
\section*{Appendix}
\label{sec:appendix}

\section{Case Study}
Although the unconfirmed transactions are not confirmed, it also contains the purpose of the user when initiating this transaction. This information is of great importance for analyzing the purpose of user behavior. In this section, we use the following two cases to illustrate the positive effect of unconfirmed transactions on the analysis of user behavior. 

\subsection{Binance Exchange Address Analysis}
\

\begin{figure*}[htbp]
    \centering
    \includegraphics[scale=0.65]{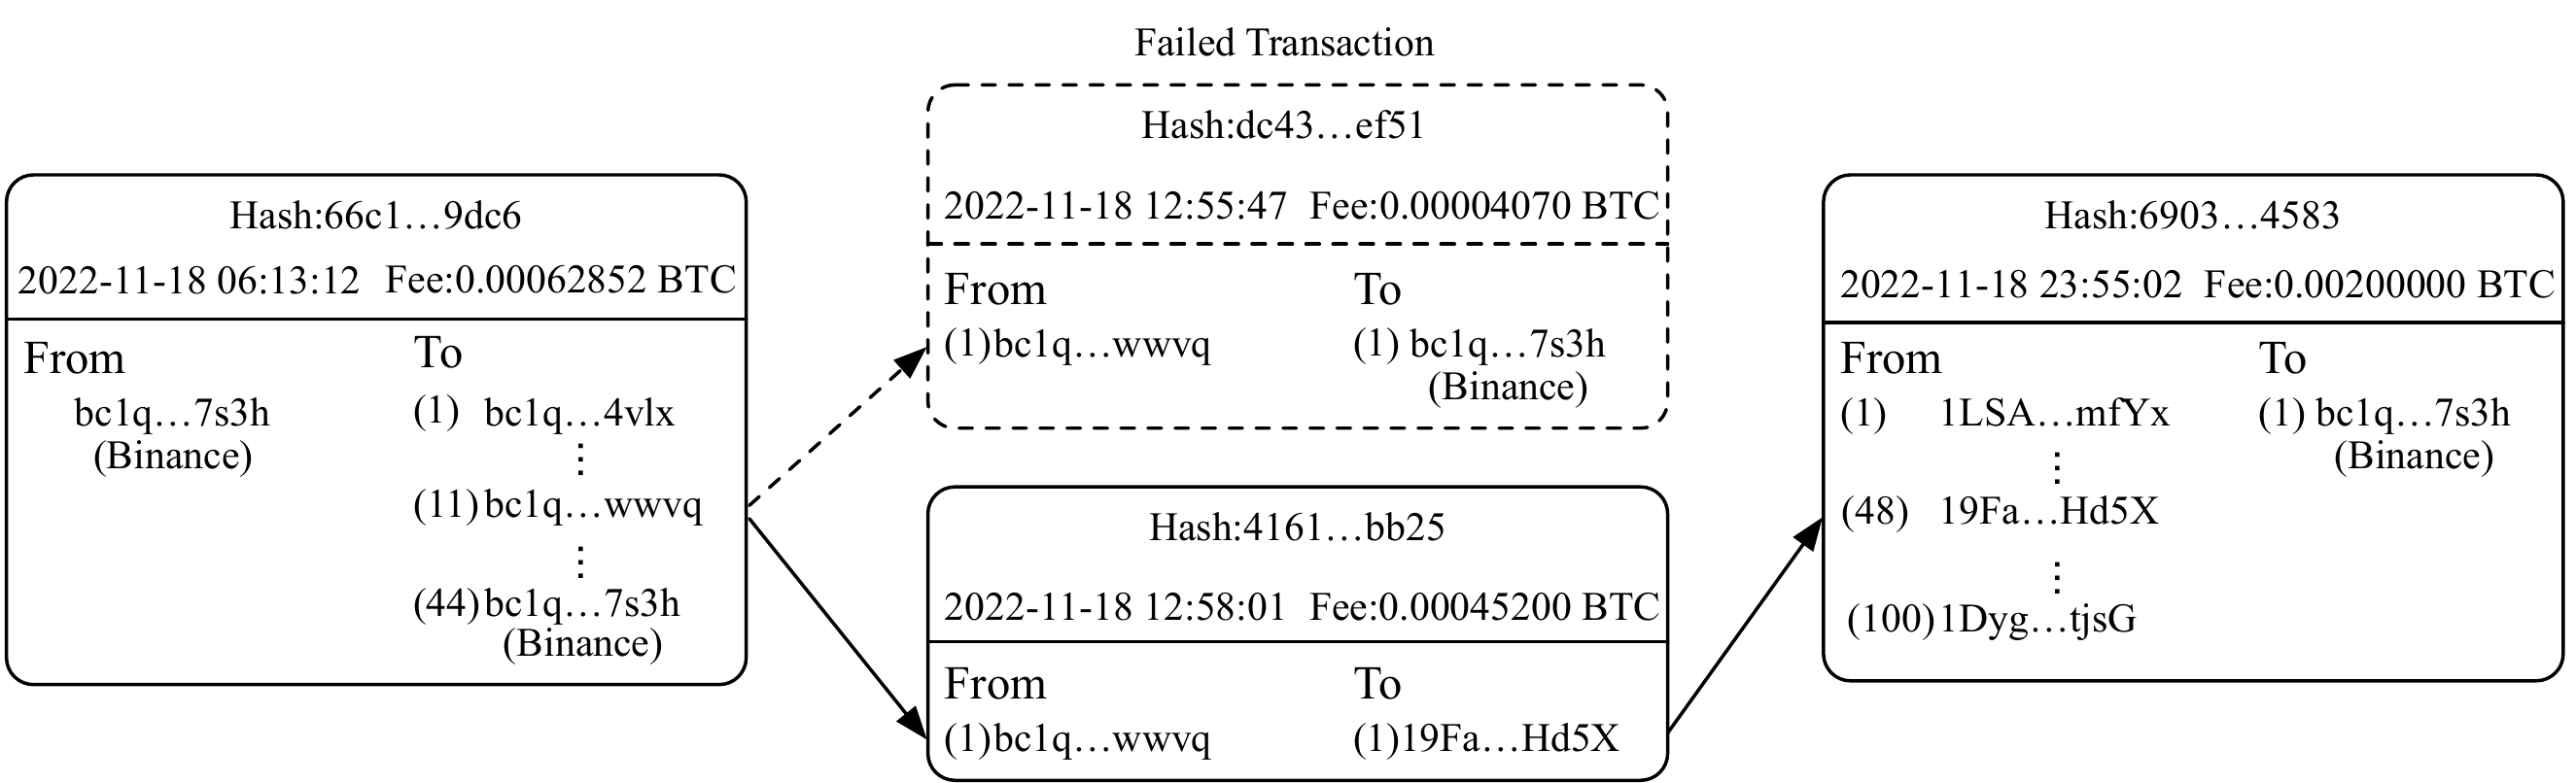}
    \caption{Binance exchange address analysis.}
    \label{fig:Binance}
\end{figure*}

One of the main safeguards used by Bitcoin exchanges to prevent attacks is the use of cold and hot storage technology within the exchange, with carefully designed risk control systems~\cite{DBLP:conf/blocksys/LiLZ19}. There are three main types of addresses controlled by Bitcoin exchanges: hot wallet addresses, cold wallet addresses and user wallet addresses.

Hot wallets are crypto wallets that are always connected to the internet. They can be mobile, desktop or web-based wallets, and are user-friendly and facilitate easy transfer of bitcoins. Private keys are kept on the app itself in hot wallets and stored online. It has hidden vulnerabilities, and hackers can target it to break into the system.  The main function of the hot wallet is to maintain a bitcoin pool for the user’s withdrawal demand. 

Cold wallets are hardware-based and exist offline. Although a cold wallet is not as convenient to use as a hot wallet, it is far more secure. Using this offline wallet keeps your keys entirely protected from online hackers. It is used to store a large number of bitcoins which received from hot wallets or other cold wallets due to the consideration of safety. Secondly, it is used to send bitcoins to hot wallets in order to keep sufficient balances.

The user wallet is created by Bitcoin exchange and the private key of the address is held by the Bitcoin exchange. Users can deposit bitcoins to Bitcoin exchange by the user wallet.

Therefore, there is a clear division of labor at addresses of a Bitcoin exchange. Figure~\ref{fig:Binance} shows a failed transaction associated with a Binance exchange, a confirmed transaction to replace the failed transaction, and another two confirmed transactions related to Binance exchange. The address \emph{bc1q...7s3h} is labeled with Binance exchange by Blockchain.com~\cite{blockchain.com}. Transaction \emph{66c1...9dc6} has 1 input and 44 outputs where Binance exchange transfers bitcoins to 44 addresses. When the transaction \emph{66c1...9dc6} is confirmed, transaction \emph{dc43...ef51} is initiated to transfer bitcoins in the address \emph{bc1q...wwvq} to Binance exchange address. Three minutes after the transaction \emph{dc43...ef51} was initiated, the transaction \emph{4161... bb25} was initiated. The second transaction spends the same UTXO as the first transaction, but has a much higher fee. As a result, miners choose the second transaction to pack into a block that is eventually confirmed. The transaction \emph{dc43...ef51} turns to be a failed transaction that is deleted by all Bitcoin nodes and can never be confirmed again. Then, another transaction \emph{6903...4583} is initiated with 100 inputs and 1 output, which transfers bitcoins in address \emph{19Fa...Hd5X} to Binance exchange address \emph{bciq...7s3h}.

In this scenario, transaction \emph{dc43...ef51} and transaction \emph{4161... bb25} are initiated by the same user because they spend the same UTXO \emph{bc1q...wwvq}. From the content of transaction \emph{dc43...ef51} and transaction \emph{6903...4583}, the purpose of the address \emph{bc1q...wwvq} is to transfer its bitcoins to Binance exchange address \emph{bc1q...7s3h}. A question worth analyzing is why the user would replace the transaction \emph{dc43...ef51} with the second one \emph{4161...bb25}.

To answer this question, we investigate 127 confirmed transactions of the address \emph{bc1q...wwvq}. All confirmed receipt transactions of the address \emph{bc1q...wwvq} are consisted of 1 input and 1 output. When the address \emph{bc1q...wwvq} transfers bitcoins to other addresses, the recipient address is always the address \emph{19Fa...Hd5X}. Then, the address \emph{19Fa...Hd5X} transfer bitcoins to Binance exchange address \emph{bc1q...7s3h}. Both transfer-in and transfer-out transactions of the address \emph{bc1q...wwvq} occur in pairs, i.e. the address receives the bitcoins and then transfers out all the bitcoins it receives. We infer that the transaction \emph{dc43...ef5} was a mistake by the Binance exchange when operating the bitcoin transfer. Address \emph{bc1q...7s3h} is a hot wallet address of Binance exchange, and under the rules of Binance exchange, address \emph{bc1q} cannot transfer bitcoins directly to address \emph{bc1q...7s3h}. Therefore, when the transaction \emph{dc43...ef51} was initiated, the operator or script discovered the misoperation and in turn initiated another high-fee transaction \emph{4161...bb25} to replace the first one.

As can be seen, the addresses controlled by the exchange all have their own roles and assume different responsibilities. The exchange works out the transaction relationships between addresses in advance, so that these addresses cannot transfer bitcoins casually between them.

Through unconfirmed transactions, we can uncover the cryptocurrency exchange's internal risk prevention and control strategies, and assist regulators in verifying the exchange's filing information and the transfer behavior inadvertently exposed by the exchange.

\subsection{Potential Dust Attack Against Whale Addresses}
\ 

\begin{figure*}[htbp]
    \centering
    \includegraphics[scale=0.55]{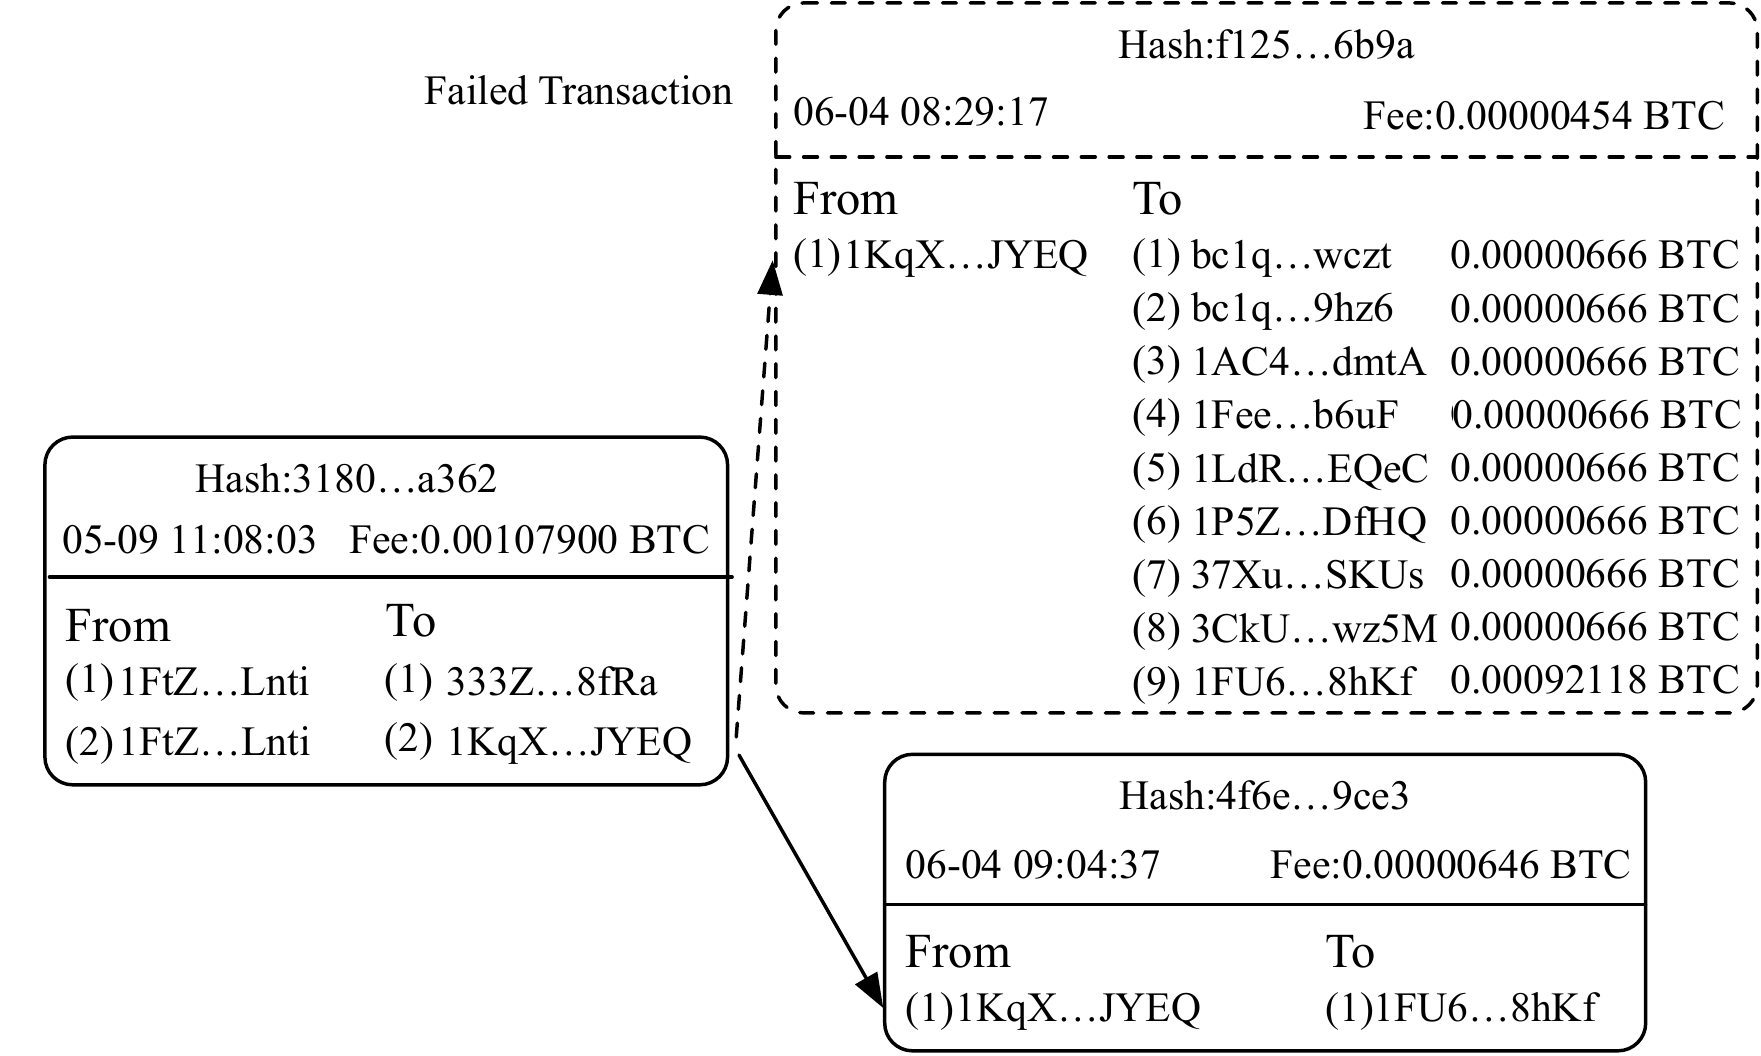}
    \caption{Potential dust attack against whale addresses.}
    \label{fig:Dust}
\end{figure*}

Dust attack can be defined as malicious behavior targeting Bitcoin users and privacy by sending tiny amounts of coins to their personal wallets~\cite{wang2018anti}. As tiny amounts will be ignored, Dust attacker’s aim in this process is to reveal the user's identity, this is done by watching and gathering information where these tiny amounts will be combined when the user does a new transaction~\cite{wang2018anti}. The transaction activity of these wallets is tracked down by the attackers in a way to link the dusted addresses and the transaction activity of these wallets in an attempt to identify the person or company behind it~\cite{wang2018anti}.

The dust attack has the following characteristics.

Small transaction value: The size of Bitcoin can be measured by BTC and satoshi, 1 satoshi = 0.00000001 BTC~\cite{DBLP:journals/fgcs/LiJCLW20}, based on the current high Bitcoin price, in order to reduce the cost of attacks, the attackers involved in the dust attack have smaller transaction value, for example 2 satoshi.

Low transaction fees: transaction fees are the costs paid by blockchain miners in both directions of transactions. In addition, considering the cost of the attack, when the attacker initiates a dust attack, the transaction fees is set to a small value and it is possible that the transaction fee can be set to zero. 

Figure~\ref{fig:Dust} shows a potential dust attack against whale addresses found in failed transactions. This figure contains 2 confirmed transactions and 1 failed transaction. In this scenario, the transaction \emph{3180...a362} is first initiated with 2 inputs and 2 outputs. When this transaction is confirmed, the address \emph{1KqX...JYEQ} transfer its received bitcoins to the address \emph{1FU6...8hKf} from the transaction \emph{4f6e...9ce3}. We can't find anything unusual about this address from confirmed transactions.

However, before the transaction \emph{4f6e...9ce3} is initiated, the transaction \emph{f125...6b9a} is first initiated. These two transactions spend the same UTXO \emph{1kqX...JYEQ}. Due to the much higher fee of transaction \emph{4f6e...9ce3}, miners choose the transaction \emph{4f6e...9ce3} to package into a block that eventually is confirmed. Therefore, the transaction \emph{f125...6b9a} turns to be a failed transaction that is deleted by all Bitcoin nodes and can never be confirmed again. The failed transaction \emph{f125...6b9a} reflect malicious behavior of the user that is not reflected in confirmed transactions.

More specifically, the transaction \emph{f125...6b9a} has 1 input and 9 outputs. It is noteworthy that all 8 outputs of this transaction have the same revenue, i.e. 0.00000666 BTC~(\$ 0.12). The remaining one output is the same as the sender address and is the change address of the sender. The address \emph{bc1q...wczt}, \emph{bc1q...9hz6} and \emph{1Fee...b6uF} are labeled with \emph{FBI3}, \emph{FBI 2~(Silk Road)} and \emph{MtGox Hacker} respectively by Blockchain.com. The stolen funds of the Bitfinex Hack 2016 continued to converge to the address \emph{bc1q...wczt}, which currently has a balance of more than 94,643 BTC without any transfers out. Nearly 70,000 bitcoins confiscated by the U.S. government from the black market site \emph{Silk Road} are transferred to the address \emph{bc1q...9hz6} in early November, 2020. as of this writing, the bitcoins have not been moved or liquidated. Former Mt.Gox CEO Mark Karpeles confirmed that the bitcoins residing at the address \emph{1Fee...b6uF} was \WCH{were} stolen from Mt.Gox exchange. The address \emph{1P5Z...DfHQ} is controlled by FTX exchange who declared bankruptcy on November 14, 2022. The other addresses except \emph{1FU6...8hKf} also have a large balance when this failed transaction \emph{f125...6b9a} is initiated. Currently, the balance of the address \emph{3CkU...wz5M} is 0. But, the balance of the address \emph{3CkU...wz5} is more than 50,620 BTC when the failed transaction \emph{f125...6b9a} is initiated. Therefore, the address \emph{1KqX...JYEQ} sends a very small amount of bitcoins to multiple whale addresses via the transaction \emph{f125...6b9a} is for a dusting attack.

When we focus only on confirmed transactions on the blockchain, we fail to discover these hidden user intents. On the one hand, unconfirmed transactions allow us to mine user privacy that confirmed transactions cannot reveal, i.e. transaction intentions. Unconfirmed transactions can also be used to identify malicious behavior that cannot be identified by confirmed transactions alone. On the other hand, unconfirmed transactions allow us to identify malicious behavior before it happens.
